# Supplementary material for: GPU Load Balancing
Source: arXiv:2212.08964 source file (2022-12-17)
Supplement: Supplementary file 1 [file appendix.tex]

%% Appendix
\appendix
\section{Appendix}
\label{sec:appendix}

Text of appendix \ldots
