# Supplementary material for: GPU Load Balancing
Source: arXiv:2212.08964 source file (2022-12-17)
Supplement: Supplementary file 2 [file appendices.tex]

\section{Appendices}

If your work needs an appendix, add it before the
``\verb|\end{document}|'' command at the conclusion of your source
document.

Start the appendix with the ``\verb|appendix|'' command:
\begin{verbatim}
  \appendix
\end{verbatim}
and note that in the appendix, chapter are lettered, not
numbered. This document has two appendices, demonstrating the chapter
and subsection identification method.
